# Supplementary material for: Bond formation insights into the Diels-Alder reaction: A bond perception and self-interaction perspective
Source: arXiv:2302.02770 ancillary file (2023-04-06)
Supplement: Supplementary file 1 [file supplementary.pdf]

# Supplementary material to

## Bond formation insights into the Diels-Alder reaction: A bond perception and self-interaction perspective

Wanja Timm Schulze,<sup>1,\*</sup> Sebastian Schwalbe,<sup>2,3,4</sup> Kai Trepte,<sup>5</sup> Alexander Croy,<sup>1</sup> Jens Kortus,<sup>2</sup> and Stefanie Gräfe<sup>1</sup>

<sup>1</sup>*Institute for Physical Chemistry, Friedrich Schiller University, Jena, 07743, Germany*

<sup>2</sup>*Institute of Theoretical Physics, TU Bergakademie Freiberg, Freiberg, 09599, Germany*

<sup>3</sup>*Center for Advanced Systems Understanding (CASUS), Görlitz, 02826, Germany*

<sup>4</sup>*Helmholtz-Zentrum Dresden-Rossendorf (HZDR), Dresden, 01328, Germany*

<sup>5</sup>*Taiwan Semiconductor Manufacturing Company North America, San Jose, USA*

(Dated: April 6, 2023)

### I. COMPUTATIONAL DETAILS

If not stated differently, the same numerical parameters as in the main manuscript are used, i.e., the SPW92 exchange-correlation functional, the double- $\zeta$  pc-1 basis set, and an unpruned grid of level 7 utilizing spin-unrestricted calculations (see Sec. 3 in the main manuscript).

### II. NUCLEAR GEOMETRY SYMMETRIES

Using LIBMSYM [1] with the same parameters as in Ref. [2], one obtains that the TS has a  $C_s$  point group, similar to comparable research [3–5]. The point group of the product cyclohexene is  $C_2$ . All the other reaction geometries have a point group of  $C_1$ , including the reactant state. The optimized fragments of the reactant state show a  $C_2$  point group for butadiene and  $D_{2h}$  for ethylene.

### III. ORBITAL LOCALIZATION

No stable minimum could be found for the IBOs using the CIAH optimizer (compare with Sec. 3 D in the main manuscript). Therefore, the implementation following Ref. [6] has been used. This implementation has no interface to obtain a Hessian, therefore no stability analysis was done for the IBOs.

### IV. DIPOLE MOMENT

The electric dipole moment  $\mu$  is defined as

$$\mu = \sum_I Z_I \mathbf{R}_I - \int d\mathbf{r} n(\mathbf{r}) \mathbf{r}, \quad (1)$$

with  $Z$  and  $\mathbf{R}$  as the charge and position of the  $I$ -th nucleus, respectively, and  $n$  as the electronic density.  $\mu$  is the absolute value of the electric dipole moment  $\mu = |\boldsymbol{\mu}|$ .

A comparison of the calculated DFT and FLO-SIC dipole moments for the separated molecules ethylene, 1,3-butadiene, and cyclohexene with experimental values can be found in Tab. I.

Table I: Calculated and experimental absolute electric dipole moments [D]. \*The experimental values use the trans structure of 1,3-butadiene, whereas the calculations use the gauche structure.

| System         | DFT  | FLO-SIC | Exp.     |
|----------------|------|---------|----------|
| ethylene       | 0.00 | 0.00    | 0 [7]    |
| 1,3-butadiene* | 0.11 | 0.02    | 0 [7]    |
| cyclohexene    | 0.37 | 0.28    | 0.55 [7] |

### V. IONIZATION POTENTIAL

Similar to the Koopmans theorem [8] in Hartree-Fock theory, the ionization potential  $E_{IP}$  in DFT can be approximated with the negative eigenenergy  $\epsilon$  of the highest occupied molecular orbital (HOMO) [9–11]

$$E_{IP} = -\epsilon. \quad (2)$$

The DFT and FLO-SIC ionization potentials  $E_{IP}$  can be found in Fig. 1. The bond formation can be seen at image 11 (TS+1), similar to the dipole moment in Fig. 6, or the UFF in Fig. 7 in the main manuscript. The corrected FLO-SIC ionization potentials are about twice as large as the DFT ionization potentials. The FLO-SIC ionization potentials are closer to experimental values than DFT (see Tab. II) but SIC over-corrects the energy.

A comparison of the calculated DFT and FLO-SIC ionization potentials for the separated molecules ethylene, 1,3-butadiene, and cyclohexene with experimental values can be found in Tab. II.

### VI. BOND PERCEPTION

The automatic bond perception, e.g., for force field calculations like the UFF is usually based on a distance criterion [18]

$$r_{ij} < r_{ij}^{EQ} + \epsilon_{th}. \quad (3)$$

\* wanja.schulze@uni-jena.de

Table II: Calculated and experimental ionization potentials [eV]. \*The experimental values use the trans structure of 1,3-butadiene, whereas the calculations use the gauche structure.

| System         | DFT FLO-SIC |       | Exp.       |            |
|----------------|-------------|-------|------------|------------|
| ethylene       | 6.90        | 12.80 | 10.50 [12] | 10.80 [13] |
| 1,3-butadiene* | 6.03        | 11.86 | 9.03 [14]  | 9.18 [15]  |
| cyclohexene    | 5.83        | 11.92 | 8.92 [16]  | 9.57 [17]  |

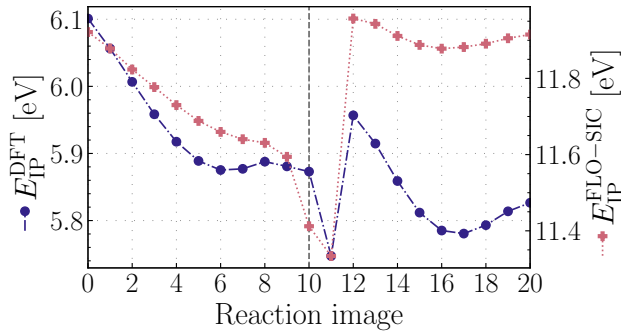

Figure 1: DFT and FLO-SIC ionization potentials  $E_{IP}$  along the reaction images. The TS is indicated at image 10 via a dashed line.

Here, the bond between atom  $i$  and  $j$  is acknowledged if the bond length  $r_{ij}$  is smaller than the sum of atomic radii  $r_i$ ,  $r_{ij}^{EQ} = r_i + r_j$ , plus a tolerance value  $\epsilon_{th}$ . Usually, covalent radii are used as atomic radii. A typical value for  $\epsilon_{th}$  is  $0.4 \text{ \AA}$  [18]. Sometimes a lower bound is used as well [19], e.g., with

$$0.8 < r_{ij} < r_{ij}^{EQ} + \epsilon_{th}. \quad (4)$$

Afterwards, the bond order of found connections will be assigned by different rules. These rules are based on basic chemical principles but require sophisticated rules and methods to accurately approximate bond orders. Possible methods are the minimization of a penalty function that is set for all atoms [18], or the evaluation of hard, length, and conjugation rules [19].

## VII. UFF CONTRIBUTIONS

The UFF energy is formed as a sum of energies of interactions [20]

$$E_{UFF} = E_R + E_\theta + E_\phi + E_\Omega + E_{vdW} + E_{el}. \quad (5)$$

Here,  $E_R$  is the bond stretching contribution,  $E_\theta$  describes the bond angle bending,  $E_\phi$  is the dihedral torsion term,  $E_\Omega$  is the inversion energy,  $E_{vdW}$  is the van der Waals interaction, and  $E_{el}$  includes electrostatic interactions. Since the UFF parameters were derived without

point charges at atom positions, the electrostatic interaction  $E_{el}$  is usually neglected [21]. The used parameterization is the same as in the original UFF description of Ref. [20].

The energy contributions of Fig. 7 in the main manuscript can be found in Fig. 2 for PYFLOSIC2 [22, 23] and in Fig. 3 for OPEN BABEL [24]. The peak at image 11 (TS+1) from Fig. 7 comes from the bond stretching term  $E_R$ . The energy barrier afterwards comes from the dihedral torsion term  $E_\phi$ . This can be explained since the approaching reactant fragments have almost reached their final distance at image 11. Afterwards, the fragments rotate against each other around the twofold rotational symmetry axis of the product. The broadening of the peak in the OPEN BABEL energies comes from a van der Waals contribution  $E_{vdW}$  at the TS.

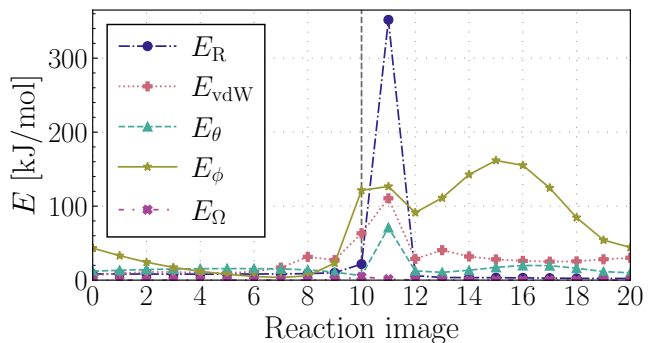

Figure 2: UFF energy contributions of the systems along the reaction images using PYFLOSIC2. The TS is indicated at image 10 via a dashed line.

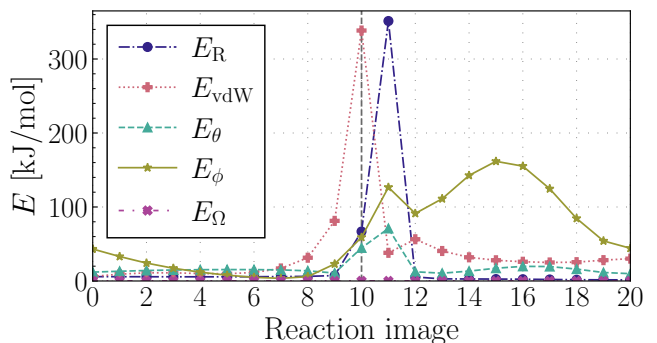

Figure 3: UFF energy contributions of the systems along the reaction images using OPEN BABEL. The TS is indicated at image 10 via a dashed line.

## VIII. ISOVALUES

To display a given density such that a certain percentage of the density is contained, an optimal isovalue has to be found. For a given `mf` SCF object coming from a DFT calculation using PYSCF [25], the script in Lst. 1 can be used to find the optimal isovalue.

Listing 1: Function to obtain the optimal isovalue that contains a certain percentage of the density.

```
def get_isovalue(mf, percent=85):
    from scipy.optimize import minimize_scalar

    dm = mf.make_rdm1()
    if dm.ndim != 2:
        dm = dm[0] + dm[1] # Density matrix for open-shell systems
    rho = mf._numint.get_rho(mf.mol, dm, mf.grids)
    n = rho @ mf.grids.weights # Integrated density

    def deviation(isovalue):
        mask = rho > isovalue
        n_mask = rho[mask] @ mf.grids.weights[mask]
        return abs(percent - (n_mask / n) * 100)

    # The isovalue is bounded by zero and the integrated density n
    res = minimize_scalar(deviation, method='bounded', bounds=[0, n])
    return res.x
```

## IX. BOND ORDER DEPENDENCE OF THE UFF ENERGY

The original UFF description provides 126 molecular mechanics (MM) types (see Sec. II. A. and Tab. I in Ref. [20]). An MM type is a specific label for an element in the periodic table, which can also include information about hybridization or geometry, the formal oxidation state, or special cases like bridging hydrogens.

Each MM type is associated with parameters used in the UFF energy expression, i.e., valence parameters (bond length  $r_i$ , bond angle  $\theta_0$ ), non-bonding parameters (distance  $x_i$ , energy  $D_i$ , scale  $\zeta$ ), and the effective charge  $Z_i$ . The bond radii  $r_{ij}$  are directly used to calculate the bond stretching energy  $E_R$

$$r_{ij} = r_i + r_j + r_{BO} + r_{EN}, \quad (6)$$

where  $r_{EN}$  is an electronegativity correction. The bond radii  $r_{ij}$  explicitly depends on the bond order  $n$  through a Pauling-type bond order correction

$$r_{BO} = 0.1332 (r_i + r_j) \ln(n). \quad (7)$$

In addition, the contributions of the bond angle bending  $E_\theta$  and the dihedral torsion  $E_\phi$  are scaled by force constants that also depend on  $r_{ij}$ .

Using PyFLOSIC2, we can use FODs or centroids to determine the bond orders for a given system. Determining the bond order of a system gives access to information about the local chemical environment of an atom in the system. With this information, one can map the bond order to a specific MM type. Consequently, the UFF energy depends directly on bond orders in the energy expressions and indirectly over the assigned MM types.

## X. SIMPLE REFERENCE MOLECULES

As we used  $d_{\max}$  in the manuscript to describe ABP distances, we have calculated three simple molecules to determine typical values for single, double, and triple bonds, seen in Fig. 4. The initial nuclear geometries for these molecules were taken from Ref. [26]. Afterwards, nuclear geometry optimizations, DFT, and FLO-SIC calculations were carried out strictly following the computational details of the main manuscript.

In ethane, there is only a C-C single bond. As expected, one observes that  $d_{\max}$  is close to zero. This represents the case where two electrons, one of each spin channel, lie directly on the bond axis. As a typical example of a C-C double bond, we used ethylene. Here,  $d_{\max}$  has an approximate value of 0.4 Å for the FODs. The distances for the FB centroids are shorter (about 0.35 Å), but close to the FODs. The centroids for the IBOs are always located on the bond axis for these systems. To get an upper limit for the double bond distances, we investigated the triple bond in acetylene. For FODs and FB, the values for  $d_{\max}$  are larger for the triple bond than for the double bond with a value of approximately 0.6 Å.

The orbital variances  $\mathcal{J}_{FB}$  have been evaluated for KSOs, FLOs, and FB orbitals in Fig. 5. The function to analyze the orbital variances follows the implementation in PYSCF. One can see that FLOs are more localized than the KSOs and thus have lower orbital variances. The FB orbital variances are similar to the FLOs but slightly less localized.

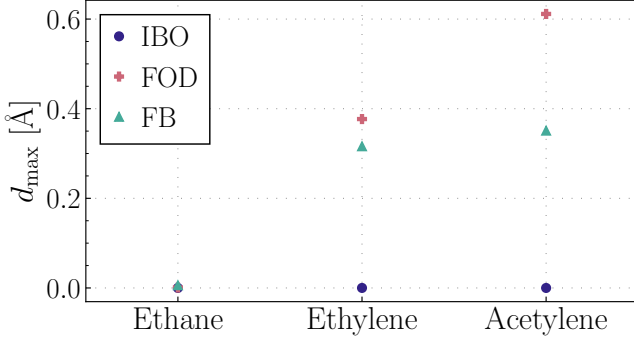

Figure 4: Maximum FOD distances  $d_{\max}$  to the C-C bond midpoint for three simple molecules.

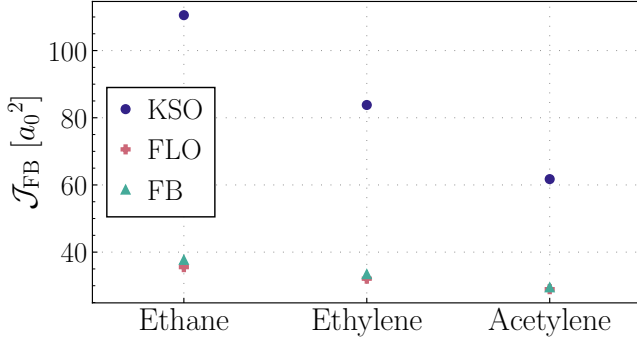

Figure 5: Orbital variances  $J_{\text{FB}}$  for occupied KSOs, FLOs, and FB orbitals for three simple molecules.

## XI. TOTAL ENERGIES

The total energies in Fig. 4a in the main manuscript were shifted by the respective total energy of the product state to bring the KS and PZ energies on a similar baseline. The unshifted values can be found in Fig. 6a for the KS energies  $E_{\text{KS}}$  and in Fig. 6b for the FLO-SIC energies  $E_{\text{PZ}}$ .

## XII. ORBITAL VARIANCES

Analog to Fig. 5 of the main manuscript, the orbital variances of all calculated localized orbitals are displayed in Fig. 7. One can clearly see that the FLOs are the most localized orbitals, having the lowest orbital variances. Similar to the trends of the main manuscript one can see two trends in the remaining orbitals. FB and ER show similar orbital variances. IBOs, PM, and generalized PM share similar orbital variances while being less localized than FB and ER orbitals. Since FB orbitals have the closest variances to the FLOs this can be seen as another indicator of why they serve as the best initial guess for FLO-SIC calculations of the investigated orbitals for this system.

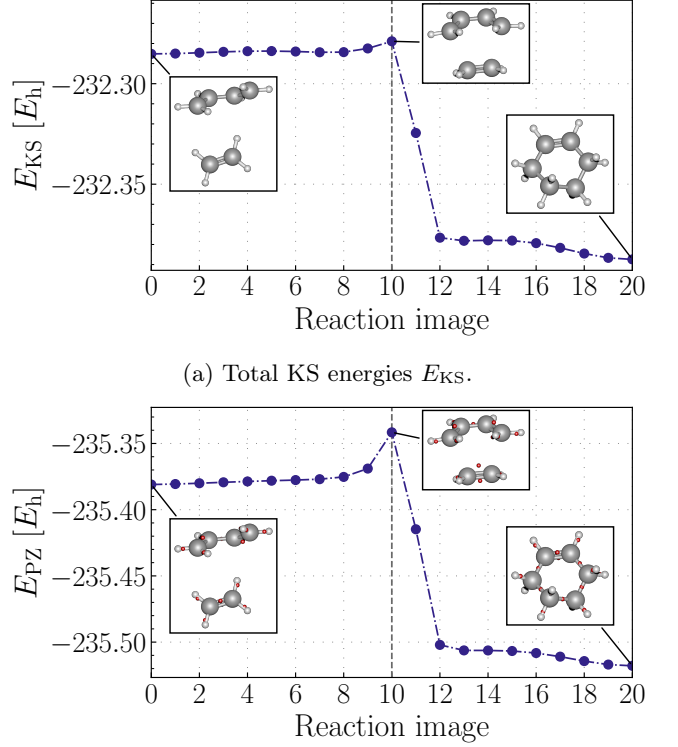

Figure 6: Energies along the reaction images. The TS is indicated at image 10 via a dashed line. The respective structures for the reactants, TS, and product are sketched in (a) and (b) accordingly, with carbon atoms colored in grey and hydrogen in white. The structures in (b) also contain the respective FOD positions in red.

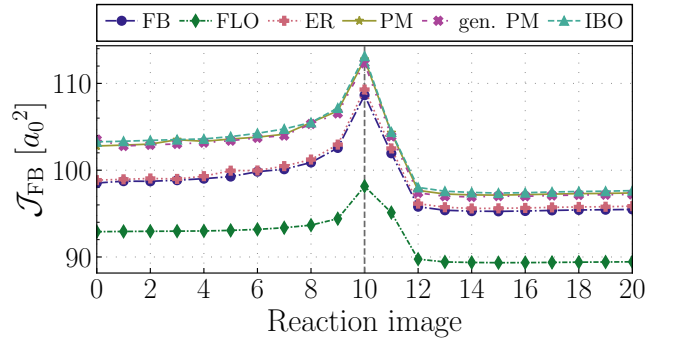

Figure 7: Orbital variances  $J_{\text{FB}}$  of occupied FLOs, IBOs, FB, ER, PM, and generalized PM orbitals along the reaction images. The TS is indicated at image 10 via a dashed line.

### XIII. COMPARISON WITH CHILLI.JL

Similar to the PYFLOSIC2 calculations that are based on PySCF, full FLO-SIC calculations have been performed using a self-written all-electron Gaussian-type orbital JULIA code called CHILLI.JL [27]. The computational parameters follow the main manuscript but differ in a few points to have additional results of different parameters. Only spin-restricted calculations were performed. A uniform grid of (75,302) has been used for all species. The atomic radii adjustment for the grid partitioning has been disabled. The scheme to generate radial grids has been changed from the Treutler-Ahlrich method [28] to the Gauss-Chebyshev method [29]. Instead of spherical Gaussian-type orbitals (GTOs), cartesian GTOs were employed. For the FOD optimization, instead of L-BFGS-B the BFGS method [30–33] has been used.

While the PYCOM method as implemented in PYFLOSIC2 utilizes a simplified stability analysis with random sampling, the JULIA variant of the method in CHILLI.JL uses a more sophisticated line search algorithm. The initial FODs were calculated with both methods separately. All sets of initial and optimized FODs follow Lewis’ theory. This hints at a higher reproducibility of the determined local minima, indicating that the presented trends are reproducible as well.

Both codes produce energies that sufficiently agree with each other. To compare the results, the mean errors (MEs) and mean absolute errors (MAEs) have been evaluated, given as

$$\text{ME} = \frac{1}{N} \sum_i (E_{i,\text{calc}} - E_{i,\text{ref}}) \quad (8)$$

$$\text{MAE} = \frac{1}{N} \sum_i |E_{i,\text{calc}} - E_{i,\text{ref}}|, \quad (9)$$

using the energies from PYFLOSIC2 as reference values. The calculated errors for the KS energies  $E_{\text{KS}}$ , the FLO-SIC energies  $E_{\text{PZ}}$ , and the SIE  $E_{\text{SI}}$  can be found in Tab. III. One can see that the DFT energies agree well below the convergence tolerance of  $1 \times 10^{-8} E_{\text{h}}$ . The FLO-SIC energy difference between both codes is about  $2 \times 10^{-5} E_{\text{h}}$ . In summary, one finds even for a different set of computational parameters that the trends of the manuscript are recovered.

Table III: Energy differences between CHILLI.JL and PYFLOSIC2 [ $E_{\text{h}}$ ].

| Energy          | ME                     | MAE                   |
|-----------------|------------------------|-----------------------|
| $E_{\text{KS}}$ | $2.91 \times 10^{-9}$  | $5.82 \times 10^{-9}$ |
| $E_{\text{PZ}}$ | $1.24 \times 10^{-5}$  | $2.20 \times 10^{-5}$ |
| $E_{\text{SI}}$ | $-2.72 \times 10^{-5}$ | $2.99 \times 10^{-5}$ |

### XIV. FUNCTIONAL DEPENDENCY

To analyze the effect of the functional, additional DFT calculations have been performed on the optimized structures, utilizing the PBEsol [34] and r<sup>2</sup>SCAN [35] functionals. The compared properties that were also investigated to track bond order changes are the maximum ABP distances  $d_{\text{max}}$  for FB orbitals, the orbital variances  $\mathcal{J}_{\text{FB}}$  of occupied FB orbitals, the total electric dipole moments  $\mu$ , and the ionization potential  $E_{\text{IP}}$  from the DFT calculations.

Most notably, the values for  $d_{\text{max}}$  (Fig. 8) show almost no dependence on the functional of choice. To simplify the figure,  $d_{\text{max}}$  has only been displayed for the C-C bond of ethylene in the reactant state since all values of  $d_{\text{max}}$  show almost no difference regardless of the choice of functional. The orbital variances  $\mathcal{J}_{\text{FB}}$  (Fig. 9) show the same trend for all functionals, while the orbital variances for PBEsol and r<sup>2</sup>SCAN are always smaller than for SPW92. Similarly, the dipole moments  $\mu$  (Fig. 10) are very similar for all functionals but show the largest differences closer to the reactant state. Larger differences can be seen in the ionization potentials  $E_{\text{IP}}$  (Fig. 11). PBEsol predicts lower ionization potentials than the already under-predicting SPW92 and r<sup>2</sup>SCAN functional. The ionization potentials SPW92 and r<sup>2</sup>SCAN have the largest difference closer to the product state. Regardless of quantitative differences, all functionals show the same qualitative trends, emphasizing that SPW92 is a valid choice for this system.

### XV. BASIS SET DEPENDENCY

Similar to functional dependency calculations above, additional DFT calculations using the family of polarization consistent basis sets pc- $n$  [36–38] have been performed. These calculations utilize the split-valence, double- $\zeta$ , triple- $\zeta$ , quadruple- $\zeta$ , and quintuple- $\zeta$  basis sets pc-0, pc-1, pc-2, pc-3, and pc-4.

Again, the choice of the basis set has almost no effect on the values of  $d_{\text{max}}$  (Fig. 12). The dipole moment  $\mu$  (Fig. 14) and the orbital variances  $\mathcal{J}_{\text{FB}}$  (Fig. 13) show larger differences the farther away one gets from the TS. This trend can also be seen in the ionization potential  $E_{\text{IP}}$  (Fig. 15). Quantitatively, all basis sets are very similar. The largest differences can be found for the pc-0 basis set, best seen in the ionization potential (Fig. 15). For the  $d_{\text{max}}$  the values for pc-0 are larger than for the bigger basis sets. Most importantly, the qualitative trends are the same for all basis sets, showing that the pc-1 basis set used in the main manuscript is sufficient for a qualitative discussion. The properties suggest that the basis set limit is almost reached at the quadruple- $\zeta$  basis set pc-3.

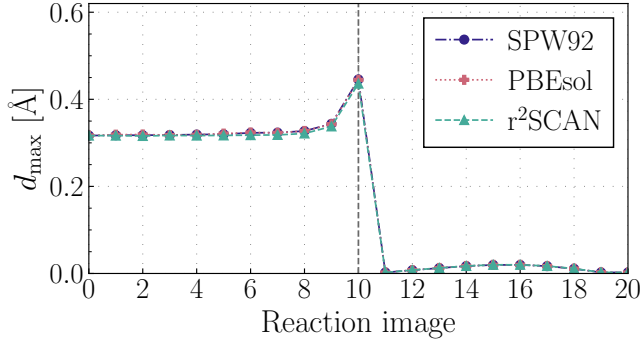

Figure 8: Maximum ABP distances  $d_{\max}$  from the C-C bond midpoints for FB orbitals. The values for different functionals are displayed as a comparison. The TS is indicated at image 10 via a dashed vertical line. Only the C-C bond for ethylene (as in the reactant state) is shown since all show almost no functional dependency.

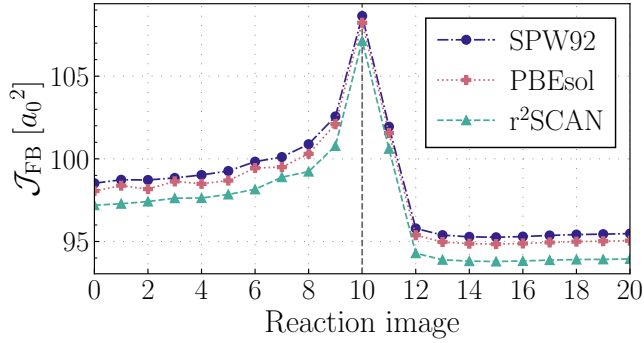

Figure 9: Orbital variances  $\mathcal{J}_{\text{FB}}$  of occupied FB orbitals along the reaction images. The values for different functionals are displayed as a comparison. The TS is indicated at image 10 via a dashed line.

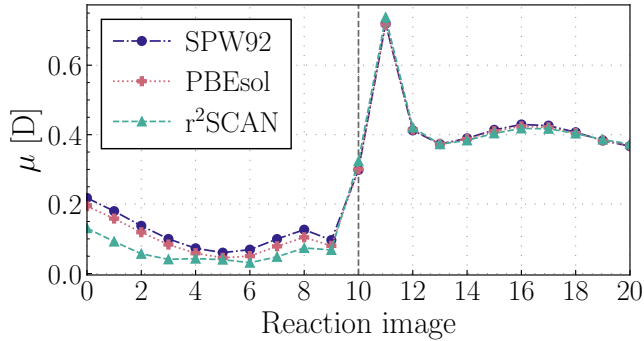

Figure 10: Absolute electric dipole moment  $\mu$  of the systems along the reaction images for the DFT densities. The values for different functionals are displayed as a comparison. The TS is indicated at image 10 via a dashed line.

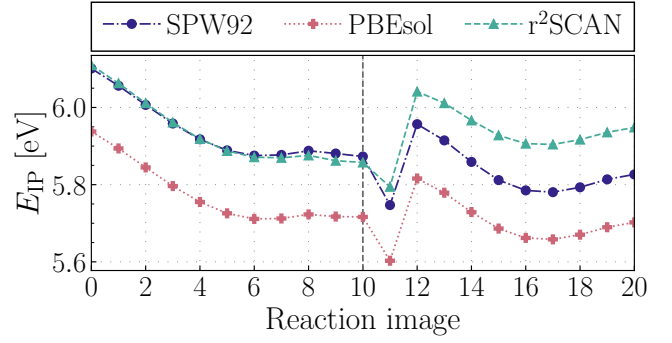

Figure 11: DFT ionization potentials  $E_{\text{IP}}$  along the reaction images. The values for different functionals are displayed as a comparison. The TS is indicated at image 10 via a dashed line.

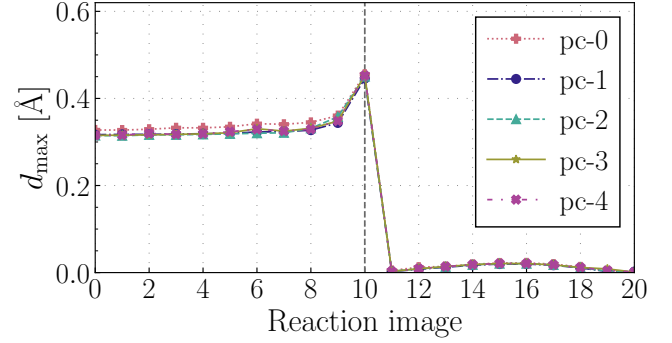

Figure 12: Maximum ABP distances  $d_{\max}$  from the C-C bond midpoints for FB orbitals. The values for different basis sets are displayed as a comparison. The TS is indicated at image 10 via a dashed vertical line. Only the C-C bond for ethylene (as in the reactant state) is shown since all show almost no basis set dependency.

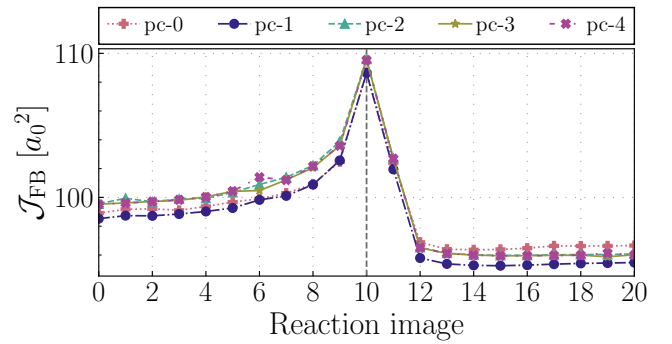

Figure 13: Orbital variances  $\mathcal{J}_{\text{FB}}$  of occupied FB orbitals along the reaction images. The values for different basis sets are displayed as a comparison. The TS is indicated at image 10 via a dashed line.

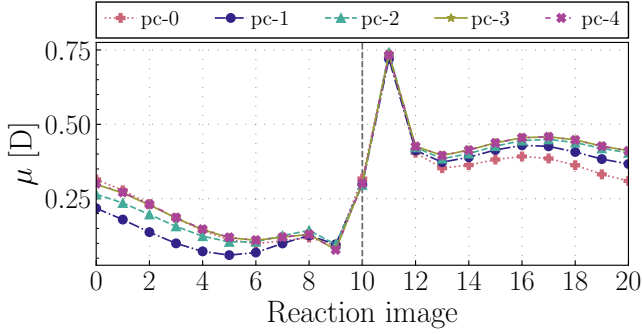

Figure 14: Absolute electric dipole moment  $\mu$  of the systems along the reaction images for the DFT densities. The values for different basis sets are displayed as a comparison. The TS is indicated at image 10 via a dashed line.

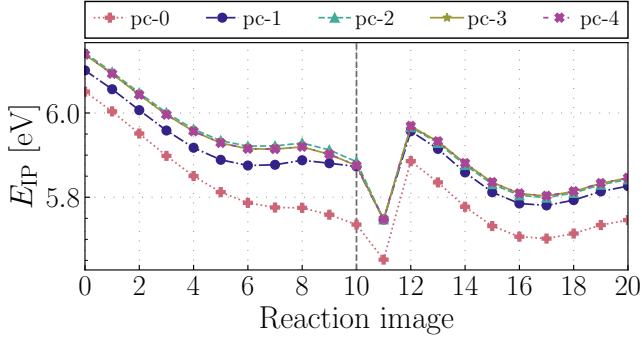

Figure 15: DFT ionization potentials  $E_{IP}$  along the reaction images. The values for different basis sets are displayed as a comparison. The TS is indicated at image 10 via a dashed line.

## XVI. MAXIMUM ABP DISTANCES

Similar to Fig. 3 in the main manuscript, the maximum ABP distance from the C-C bond axis  $d_{\max}$  has been plotted for all double bonds. The centroids for the FLOs (Fig. 16), FB (Fig. 17), and ER (Fig. 18) show a similar trend to the FODs of Fig. 3 in the main manuscript. The distance  $d_{\max}$  is almost constant at about 0.35 Å before reaching its peak at the TS and becoming close to zero afterwards when forming a single bond. For the FB orbitals,  $d_{\max}$  for the double bonds is slightly larger than for ER and therefore a slightly better approximation to the FODs.

For PM (Fig. 19), generalized PM (Fig. 20), and IBOs (Fig. 21),  $d_{\max}$  is close to zero not only for the single bond but for the double bond as well, with a distance usually between 0.05 Å and 0.1 Å. Due to this, these centroids are not a satisfactory approximation for the FODs. Still, the TS is very distinguishable forming a distinct peak for the double bonds in the reactants.

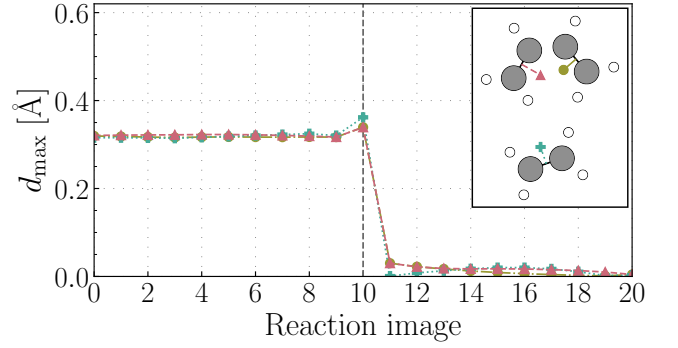

(a) Maximum FLO centroid distances for the breaking double bonds.

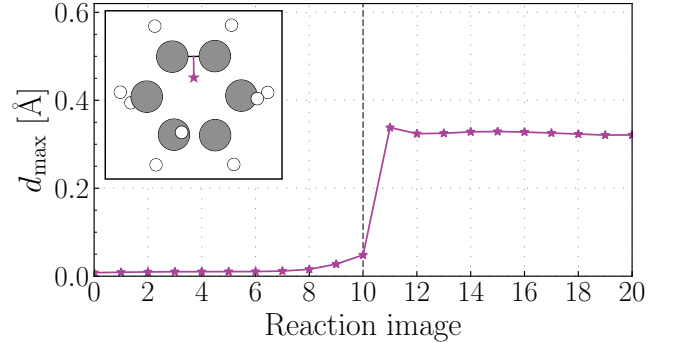

(b) Maximum FLO centroid distances for the forming double bond.

Figure 16: Maximum FLO centroid distances  $d_{\max}$  from the C-C midpoints that form double bonds. The TS is indicated at image 10 via a dashed vertical line. The color-coded centroid positions in the molecule are indicated.

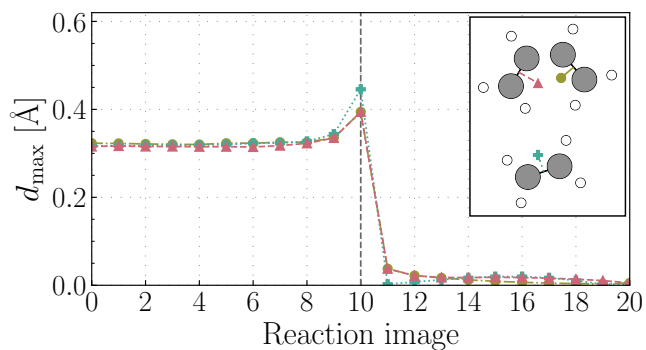

(a) Maximum FB centroid distances for the breaking double bonds.

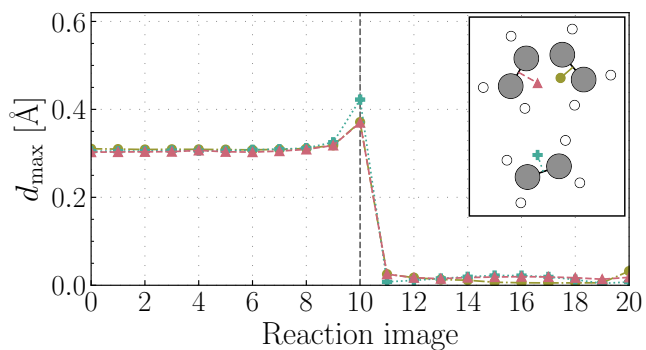

(a) Maximum ER centroid distances for the breaking double bonds.

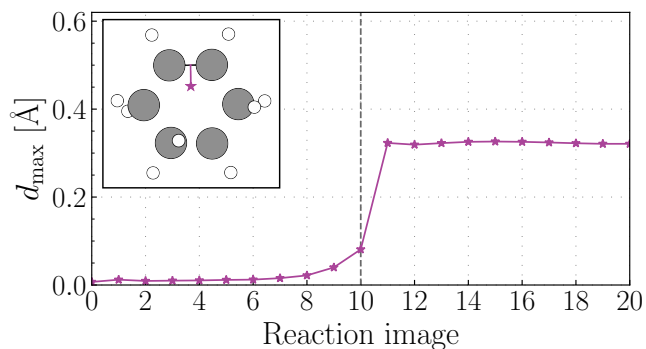

(b) Maximum FB centroid distances for the forming double bond.

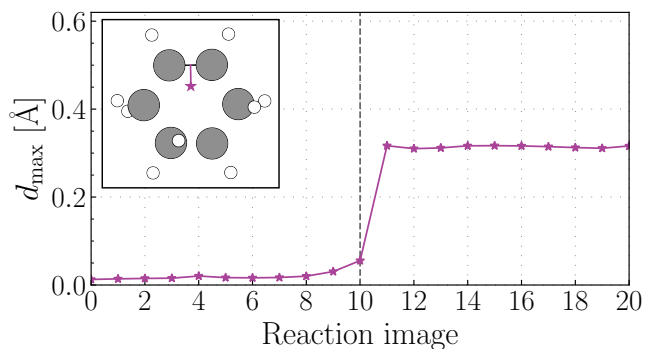

(b) Maximum ER centroid distances for the forming double bond.

Figure 17: Maximum FB centroid distances  $d_{\max}$  from the C-C midpoints that form double bonds. The TS is indicated at image 10 via a dashed vertical line. The color-coded centroid positions in the molecule are indicated.

Figure 18: Maximum ER centroid distances  $d_{\max}$  from the C-C midpoints that form double bonds. The TS is indicated at image 10 via a dashed vertical line. The color-coded centroid positions in the molecule are indicated.

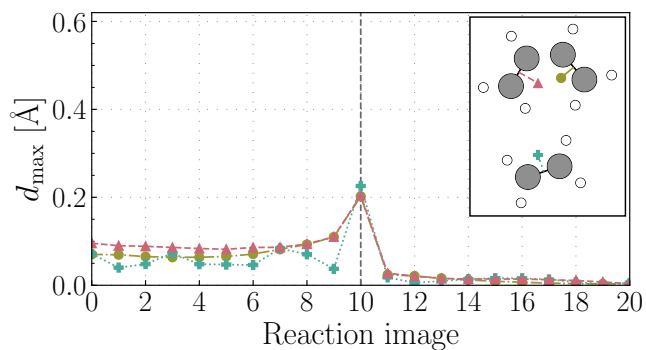

(a) Maximum PM centroid distances for the breaking double bonds.

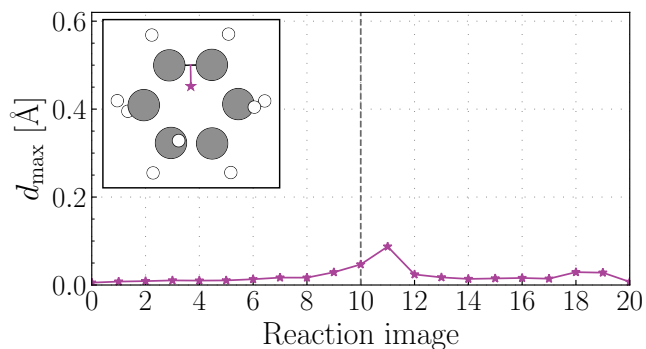

(b) Maximum PM centroid distances for the forming double bond.

Figure 19: Maximum PM centroid distances  $d_{\max}$  from the C-C midpoints that form double bonds. The TS is indicated at image 10 via a dashed vertical line. The color-coded centroid positions in the molecule are indicated.

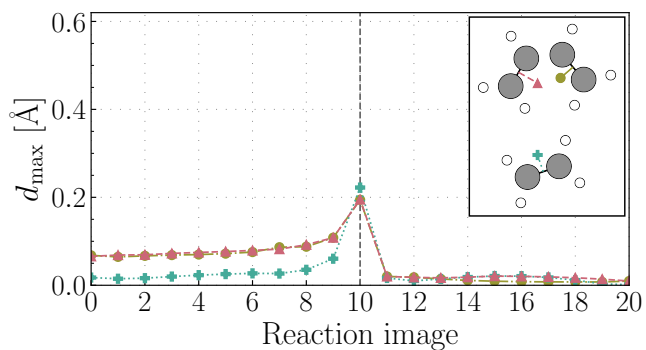

(a) Maximum generalized PM centroid distances for the breaking double bonds.

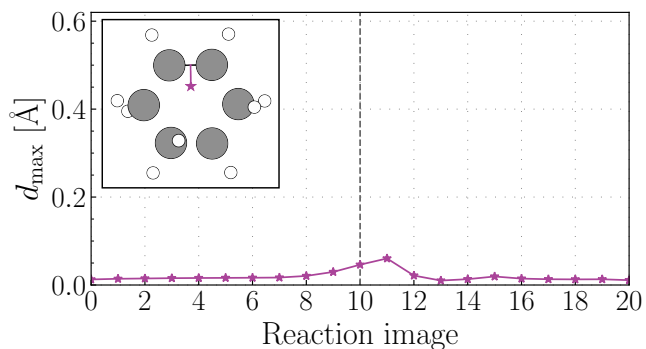

(b) Maximum generalized PM centroid distances for the forming double bond.

Figure 20: Maximum generalized PM centroid distances  $d_{\max}$  from the C-C midpoints that form double bonds. The TS is indicated at image 10 via a dashed vertical line. The color-coded centroid positions in the molecule are indicated.

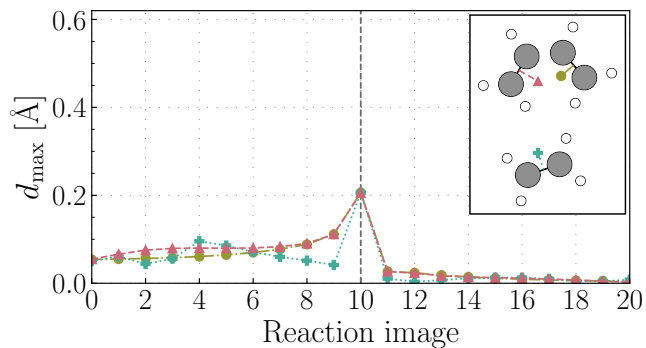

(a) Maximum IBO centroid distances for the breaking double bonds.

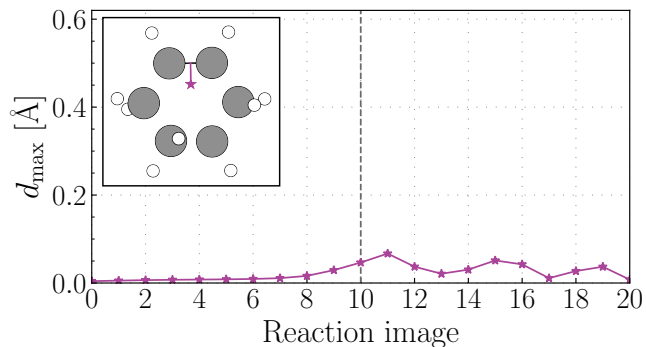

(b) Maximum IBO centroid distances for the forming double bond.

Figure 21: Maximum IBO centroid distances  $d_{\max}$  from the C-C midpoints that form double bonds. The TS is indicated at image 10 via a dashed vertical line. The color-coded centroid positions in the molecule are indicated.

## XVII. CENTROIDS FOR SELECTED IMAGES

In the following, the centroids for FLOs (Fig. 22), FB (Fig. 23), ER (Fig. 24), PM (Fig. 25), generalized PM (Fig. 26), and IBOs (Fig. 27) have been displayed, similar to Fig. 2 in the main manuscript. In the case of nearly identical centroids, only one spin channel has been displayed.

For FLOs, FB, and ER one can see a similar picture to the FODs. Both centroids are well separated around the C-C bond midpoints. This can not be said for PM, generalized PM, and IBOs, where the centroids are close to the bond axis. This can be ideally observed for the centroids of ethylene in the TS (Fig. 27b) or at the double bond in TS+1 (Fig. 27c).

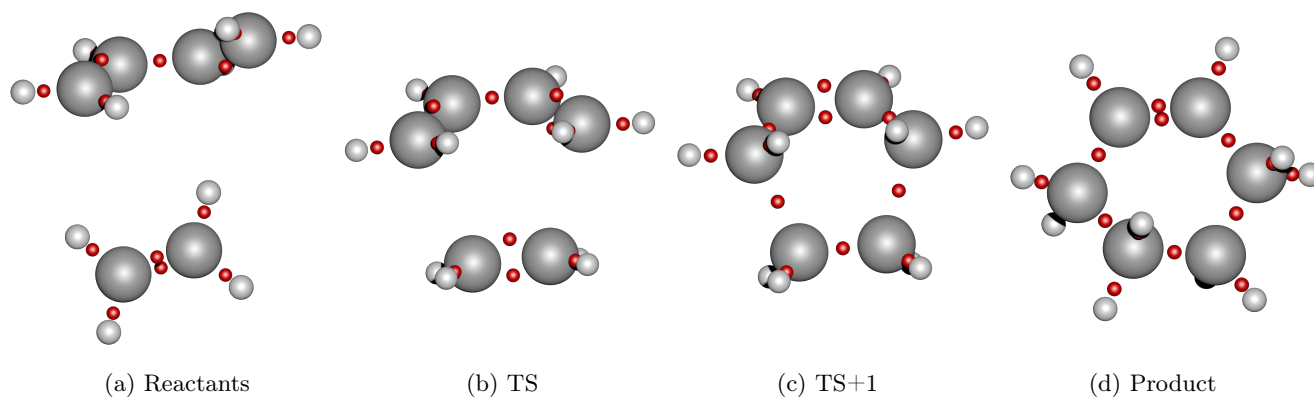

Figure 22: FLO centroids (red) for the reactants, the TS, the image after the TS (TS+1), and the product. Only one spin channel has been displayed since the centroid positions for these images coincide for both spin channels.

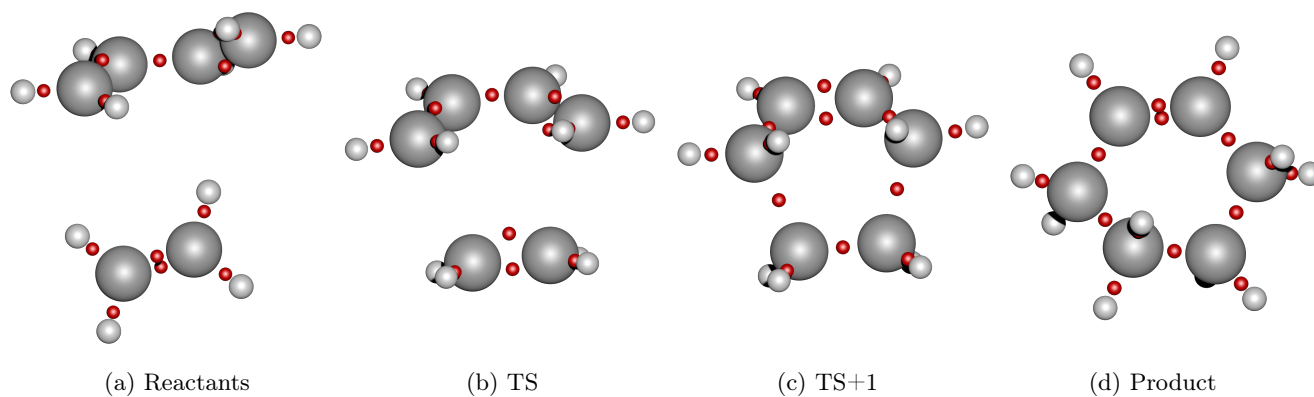

Figure 23: FB centroids (red) for the reactants, the TS, the image after the TS (TS+1), and the product. Only one spin channel has been displayed since the centroid positions for these images coincide for both spin channels.

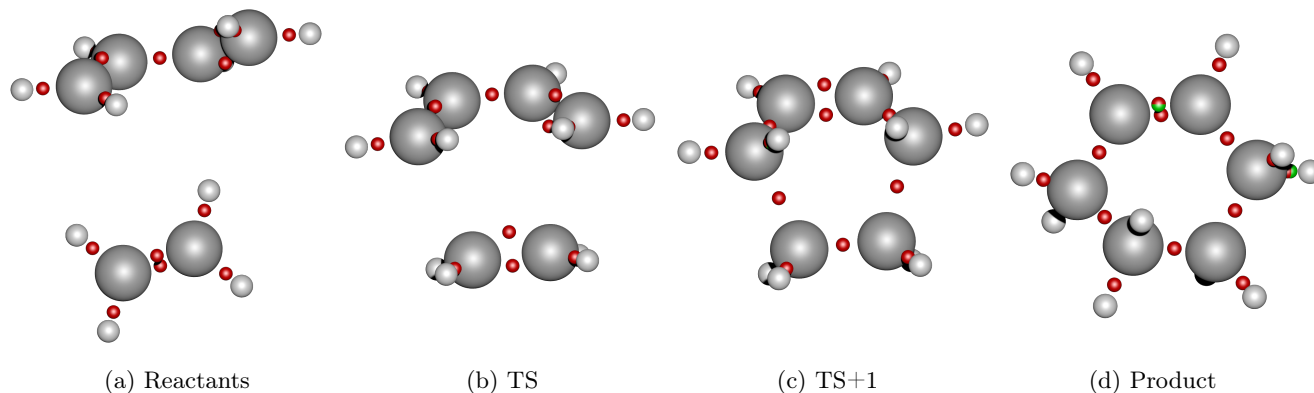

Figure 24: ER centroids (red) for the reactants, the TS, the image after the TS (TS+1), and the product. If the centroid distance between both spin channels is larger than 0.1 Å the centroid of the second spin channel will be displayed in green.

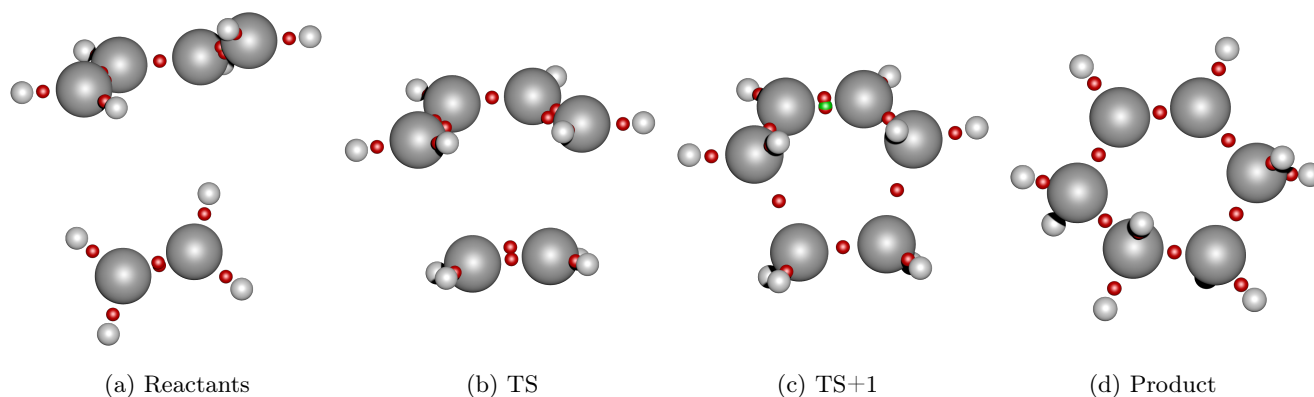

Figure 25: PM centroids (red) for the reactants, the TS, the image after the TS (TS+1), and the product. If the centroid distance between both spin channels is larger than 0.1 Å the centroid of the second spin channel will be displayed in green.

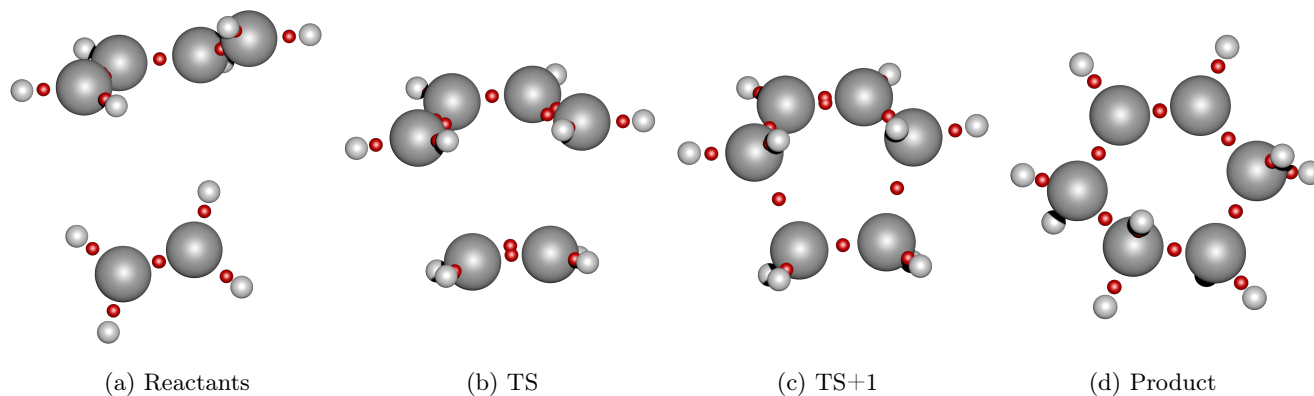

Figure 26: Generalized PM centroids (red) for the reactants, the TS, the image after the TS (TS+1), and the product. Only one spin channel has been displayed since the centroid positions for these images coincide for both spin channels.

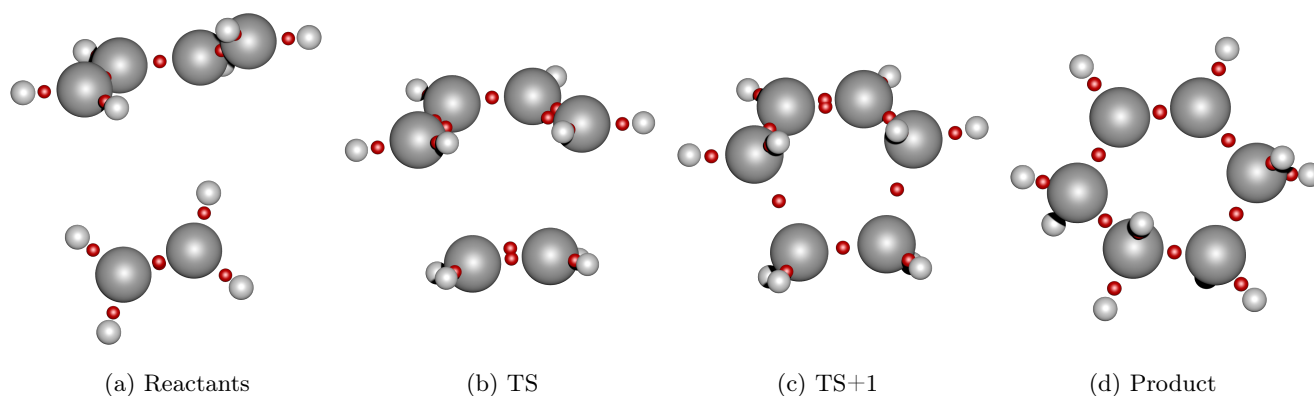

Figure 27: IBO centroids (red) for the reactants, the TS, the image after the TS (TS+1), and the product. Only one spin channel has been displayed since the centroid positions for these images coincide for both spin channels.

## REFERENCES

- [1] M. Johansson and V. Veryazov, Automatic procedure for generating symmetry adapted wavefunctions, *J. Cheminf.* **9**, 8 (2017).
- [2] K. Treppe, S. Schwalbe, S. Liebing, W. T. Schulze, J. Kortus, H. Myneni, A. V. Ivanov, and S. Lehtola, Chemical bonding theories as guides for self-interaction corrected solutions: Multiple local minima and symmetry breaking, *J. Chem. Phys.* **155**, 224109 (2021).
- [3] K. N. Houk, Y. T. Lin, and F. K. Brown, Evidence for the concerted mechanism of the Diels-Alder reaction of butadiene with ethylene, *J. Am. Chem. Soc.* **108**, 554 (1986).
- [4] F. Bernardi, A. Bottoni, M. J. Field, M. F. Guest, I. H. Hillier, M. A. Robb, and A. Venturini, MC-SCF study of the Diels-Alder reaction between ethylene and butadiene, *J. Am. Chem. Soc.* **110**, 3050 (1988).
- [5] E. Goldstein, B. Beno, and K. N. Houk, Density Functional Theory Prediction of the Relative Energies and Isotope Effects for the Concerted and Stepwise Mechanisms of the Diels-Alder Reaction of Butadiene and Ethylene, *J. Am. Chem. Soc.* **118**, 6036 (1996).
- [6] G. Knizia, Intrinsic Atomic Orbitals: An Unbiased Bridge between Quantum Theory and Chemical Concepts, *J. Chem. Theory Comput.* **9**, 4834 (2013).
- [7] R. D. Nelson, D. R. Lide, and A. A. Maryott, *Selected Values of Electric Dipole Moments for Molecules in the Gas Phase*, NBS National Standard Reference Data Series No. 10 (U.S. National Bureau of Standards, 1967).
- [8] T. Koopmans, Über die Zuordnung von Wellenfunktionen und Eigenwerten zu den Einzelnen Elektronen Eines Atoms, *Physica* **1**, 104 (1934).
- [9] J. P. Perdew, R. G. Parr, M. Levy, and J. L. Balduz, Density-Functional Theory for Fractional Particle Number: Derivative Discontinuities of the Energy, *Phys. Rev. Lett.* **49**, 1691 (1982).
- [10] M. Levy, J. P. Perdew, and V. Sahni, Exact differential equation for the density and ionization energy of a many-particle system, *Phys. Rev. A* **30**, 2745 (1984).
- [11] J. P. Perdew and M. Levy, Comment on "Significance of the highest occupied Kohn-Sham eigenvalue", *Phys. Rev. B* **56**, 16021 (1997).
- [12] K. V. Wood and J. W. Taylor, A photoionization mass spectrometric study of autoionization in ethylene and trans-2-butene, *Int. J. Mass Spectrom. Ion Phys.* **30**, 307 (1979).
- [13] P. Kusch, A. Hustrulid, and J. T. Tate, The Dissociation of HCN, C<sub>2</sub>H<sub>2</sub>, C<sub>2</sub>N<sub>2</sub> and C<sub>2</sub>H<sub>4</sub> by Electron Impact, *Phys. Rev.* **52**, 843 (1937).
- [14] G. Bieri, F. Burger, E. Heilbronner, and J. P. Maier, Valence Ionization Energies of Hydrocarbons, *Helv. Chim. Acta* **60**, 2213 (1977).
- [15] H. Bock and H. Seidl, "d-Orbital effects" in silicon-substituted  $\pi$ -electron systems. XI. Syntheses and properties of the isomeric bis(trimethylsilyl)-1,3-butadienes, *J. Am. Chem. Soc.* **90**, 5694 (1968).
- [16] D. A. Dimeo and A. J. Yencha, Photoelectron Spectra of Bicyclic and Exocyclic Olefins, *J. Chem. Phys.* **53**, 4536 (1970).
- [17] M.-T. Praet, Ionisation et Dissociation du 1-Méthylcyclopentène, du Méthylèncyclopentane et de quelques Isomères par impact d'Electrons et de Photons, *Org. Mass Spectrom.* **4**, 65 (1970).
- [18] S. Artemova, L. Jaillet, and S. Redon, Automatic molecular structure perception for the universal force field, *J. Comput. Chem.* **37**, 1191 (2016).
- [19] Q. Zhang, W. Zhang, Y. Li, J. Wang, L. Zhang, and T. Hou, A rule-based algorithm for automatic bond type perception, *J. Cheminf.* **4**, 26 (2012).
- [20] A. K. Rappe, C. J. Casewit, K. S. Colwell, W. A. Goddard, and W. M. Skiff, UFF, a full periodic table force field for molecular mechanics and molecular dynamics simulations, *J. Am. Chem. Soc.* **114**, 10024 (1992).
- [21] L. Jaillet, S. Artemova, and S. Redon, IM-UFF: Extending the universal force field for interactive molecular modeling, *J. Mol. Graph. Model.* **77**, 350 (2017).
- [22] S. Schwalbe, L. Fiedler, J. Kraus, J. Kortus, K. Treppe, and S. Lehtola, PyFLOSIC: Python-based Fermi-Löwdin orbital self-interaction correction, *J. Chem. Phys.* **153**, 084104 (2020).
- [23] S. Liebing, K. Treppe, and S. Schwalbe, Effect of Molecular and Electronic Geometries on the Electronic Density in FLO-SIC, in *Springer Proceedings in Physics* (Springer International Publishing, 2022) pp. 167–186.
- [24] N. M. O'Boyle, M. Banck, C. A. James, C. Morley, T. Vandermeersch, and G. R. Hutchison, Open Babel: An open chemical toolbox, *J. Cheminf.* **3**, 33 (2011).
- [25] Q. Sun *et al.*, Recent developments in the PySCF program package, *J. Chem. Phys.* **153**, 024109 (2020).
- [26] P. Linstrom, NIST Chemistry WebBook, NIST Standard Reference Database 69 (1997).
- [27] S. Schwalbe, K. Treppe, and W. T. Schulze, chilli.jl [chilli\_jl] (2023).
- [28] O. Treutler and R. Ahlrichs, Efficient molecular numerical integration schemes, *J. Chem. Phys.* **102**, 346 (1995).
- [29] M. Krack and A. M. Köster, An adaptive numerical integrator for molecular integrals, *J. Chem. Phys.* **108**, 3226 (1998).
- [30] C. G. Broyden, The Convergence of a Class of Double-rank Minimization Algorithms 1. General Considerations, *IMA J. Appl. Math.* **6**, 76 (1970).
- [31] R. Fletcher, A new approach to variable metric algorithms, *Comput. J.* **13**, 317 (1970).
- [32] D. Goldfarb, A family of variable-metric methods derived by variational means, *Math. Comp.* **24**, 23 (1970).
- [33] D. F. Shanno, Conditioning of quasi-Newton methods for function minimization, *Math. Comp.* **24**, 647 (1970).
- [34] J. P. Perdew, A. Ruzsinszky, G. I. Csonka, O. A. Vydrov, G. E. Scuseria, L. A. Constantin, X. Zhou, and K. Burke, Restoring the Density-Gradient Expansion for Exchange in Solids and Surfaces, *Phys. Rev. Lett.* **100**, 136406 (2008).
- [35] J. W. Furness, A. D. Kaplan, J. Ning, J. P. Perdew, and J. Sun, Accurate and Numerically Efficient r<sup>2</sup>SCAN Meta-Generalized Gradient Approximation, *J. Phys. Chem. Lett.* **11**, 8208 (2020).
- [36] F. Jensen, Polarization consistent basis sets: Principles, *J. Chem. Phys.* **115**, 9113 (2001).
- [37] F. Jensen, Polarization consistent basis sets. II. Estimating the Kohn-Sham basis set limit, *J. Chem. Phys.* **116**, 7372 (2002).
- [38] F. Jensen, Polarization consistent basis sets. III. the importance of diffuse functions, *J. Chem. Phys.* **117**, 9234 (2002).
